# Supplementary material for: A Spectral Condition for Feature Learning
Source: arXiv:2310.17813 source file (2024-05-14)
Supplement: Supplementary file 1 [file comparison_appendix.tex]

\section{Contrast with popular parametrizations}
\label{app:comparison}

We have shown that training in accordance with our \textit{spectral scaling condition} (\cref{cond:scaling}) at every layer suffices to achieve correctly-scaled feature evolution, and we have given width scalings for layerwise hyperparameters --- specifically, each layer's initialization scale $\sigma_\ell$ and learning rate --- that suffice to put this condition into action in a standard deep learning paradigm.
These hyperparameter scalings together constitute a \textit{parametrization} for a deep neural network.
Here we compare our ``spectral parametrization'' with popular parametrizations.
We find that our parametrization recovers the ``maximal update parametrization'' (\muP{}) at all layers in a unifying manner.
We point out differences with other parametrizations and leverage our spectral language to show that all but \muP{} violate \cref{des:scaling}.

\subsection{Comparison with the ``maximal update parametrization''}

The maximal update parametrization (\muP{}) of has been recently proposed as a scaling rule which retains feature learning even at infinite width.
% , a claim which is validated by experiments transferring hyperparameters from small to large width [CITATION].
Direct comparison between our spectral parametrization (\cref{claim:spectral_pzn}) and the scaling tables for MLPs reported by \citet{Yang2021TensorPI} and \citet{yang:2022-tp5} reveals that we have recovered \muP{}.
Satisfyingly, we have done so in a unifying manner across layers: while said tables report different scalings for the first, hidden, and final layers, we give a \textit{single expression per hyperparameter} which depends solely on a layer's fan-in and fan-out dimensions.
Our universal expressions for $\sigma_\ell$ and $\eta_\ell$ recover these three cases when taking all hidden layer widths uniformly to infinity while keeping input and output dimension finite.
Our parametrization also includes scaling with respect to the input dimension $d_0$ and output dimension $d_L$ (as opposed to neglecting them as agnostic $\Theta(1)$ quantities) and prescribes adaptations for hidden widths which are not uniform (i.e. $d_{\ell-1} \neq d_\ell$) and thus in fact slightly \textit{generalizes} \muP{}.
We note that \muP{} has been shown to induce both feature learning and optimal hyperparameter scaling with respect to width where other parametrizations do not \citep{yang:2022-tp5, dey:2023-cerebras-gpt}, and these experiments serve to validate our spectral analysis and proposed scaling rules.

We note that our spectral language sheds much light on \textit{why} \muP{} achieves feature learning.
For example: if the prescribed learning rates were any different, then the updates would be too big or too small (violating \cref{cond:scaling}), and the subsequent feature updates would vanish or explode (violating \cref{des:scaling}).
It bears noting that $\norm{\DW_\ell}_*$ is in this sense ``as big as it can be'' without feature blowup, and this is precisely what is meant by ``maximal'' in ``maximal update parametrization.''

Perhaps the most unintuitive feature of \muP{} is the fact that the final layer is smaller at initialization than in other parametrizations (in particular, it is smaller by a factor of $1 / \sqrt{d_{\ell-1}}$).
Our spectral analysis gives an intuitive reason for this: the spectral norm of $\mW_L$ must satisfy \cref{cond:scaling} at initialization, because were it any bigger, then feature updates $\Delta \vh_{L-1}(\vx)$ which satisfy \cref{des:scaling} would be so big as to cause blowup in the network output.
Other initialization schemes --- which naively take $\sigma_\ell = \Theta(1 / \sqrt{d_{\ell-1}})$ at all layers and neglect the second argument to the $\min$ in \cref{claim:spectral_pzn} --- are thus doomed at initialization to have vanishing feature evolution because their final layers are too large.

Finally, we note that the formal derivation of \muP{} via the ``Tensor Programs'' framework given by \citet{Yang2021TensorPI}, while mathematically rigorous, is rather technical and requires nontrivial unpacking to understand.
One may view a main contribution of the present work as providing a (nonrigorous) spectral derivation of \muP{} which is more accessible and more clearly delivers key intuitions.
We suggest that beginners to \muP{} use this work as a first reference.

\subsection{Contrast to ``standard parametrization''}

At the time of writing, the vast majority of deep learning systems in practice use a ``standard parametrization'' (SP) in which layerwise initialization and learning rates scale as
\begin{equation}
    \sigma_\ell = \Theta(1 / \sqrt{d_{\ell-1}})
    \qquad
    \text{and}
    \qquad
    \eta_\ell = \eta.
\end{equation}
That is, the initialization scale differs from ours in layers with fan-out smaller than fan-in, and the learning rate is viewed as a constant across layers.
This initialization scheme is often referred to as ``Kaiming,'' ``Xavier,'' or ``LeCun'' initialization \citep{he:2015-delving-deep-into-rectifiers, glorot:2010-difficulty-of-training-deep-nets, lecun:2002-backprop-tricks}.
This parametrization is currently the default in PyTorch \citep{paszke:2019-pytorch}.

As discussed in the previous subsection, the last-layer initialization in the SP is too large, and we are doomed from the start to see either negligible hidden vector evolution or exploding network output once network width is sufficiently large.
The SP can in fact be worse than this: $\eta$ is typically viewed as a $\Theta(1)$ quantity (which inevitably leads to output blowup at large width).
Even if it is scaled inversely with width, the existence of one global $\eta$ means that \textit{at least} updates to the first layer $\DW_1$ will have vanishing effect on the output at large width.

\subsection{Contrast to ``neural tangent parametrization''}

The neural tangent parametrization (NTP) of \citep{jacot:2018, lee:2019-ntk} fixes the learning rate scaling of the SP (so that training at all layers changes the network output without causing blowup).%
\footnote{For an MLP with uniform hidden layer width $d$, the NTP is equivalent to the SP with $\eta = \Theta(1/d)$ except at the first layer.}
However, for the aforementioned reasons, the last-layer initialization scale is still incorrect for seeing leading-order feature evolution at earlier layers.

\subsection{Contrast to ``Frobenius-normalized updates''}

A basic consequence of \cref{cond:scaling} is the requirement that the spectral norm of the update at layer $\ell$ be proportional to the spectral norm of the weight matrix to which it is applied: $\norm{\DW_\ell}_* \propto \norm{\mW_\ell}_*$. This is in contrast to a body of optimization work \cite{You:EECS-2017-156, my-fromage, my-madam, my-nero} that has required rather that the \textit{Frobenius norm} of the update at layer $\ell$ be proportional to the \textit{Frobenius norm} of the weight matrix to which it is applied: $\norm{\DW_\ell}_F \propto \norm{\mW_\ell}_F$. For instance, \citet{my-fromage} analysed the operator structure of deep neural networks and wrote down perturbation bounds on network activations in terms of perturbations to the weight matrices at each layer, and used these perturbation bounds to motivate making updates that are small in Frobenius norm. The flaw in that analysis is the assumption that weight matrices and their perturbations have identical conditioning structure (Condition 2 of Theorem 1 in \citep{my-fromage}). If, instead, we assume that perturbations have low stable rank $\smash{\norm{\DW_\ell}_F^2 /\norm{\DW_\ell}_*^2 \approx 1}$ while weight matrices have high stable rank $\smash{\norm{\mW_\ell}_F^2 /\norm{\mW_\ell}_*^2 \approx \min(d_\ell,d_{\ell -1})}$, then \cref{cond:scaling} implies a form of \textit{width-corrected Frobenius-normalized update}: $\smash{\norm{\DW_\ell}_F \propto \norm{\mW_\ell}_F / \sqrt{\min(d_\ell, d_{\ell-1})}}$.
